# Supplementary material for: Emergence of Metcalfe's Law: Mechanism and Model
Source: arXiv:2312.11110 source file (2024-07-11)
Supplement: Supplementary file 1 [file appendix.tex]

\subsection{Some Basic Lemmas}
\begin{lem}[Minimal Spanning Tree \cite{steele1988growth}]\label{lem-growthsteel}
	Let $X_i$, $1\leq i <\infty$, denote independent random variables with
	values in $\mathbb{R}^d$, $d\geq 2$, and let $M_n$ denote the cost of
	a minimal spanning tree of a complete graph with vertex set $\{X_i\}_{i=1}^n$, where the cost of an edge $(X_i, X_j)$ is given by $\Psi((|X_i-X_j|))$.
	Here, $|X_i-X_j|$ denotes the Euclidean distance between $X_i$ and $X_j$ and
	$\Psi$ is a monotone function. For bounded random variables and $0<\sigma<d$,
	it holds that as $n\to \infty$, with probability $1$, one has
	\[
	M_n\sim c_1(\sigma,d)\cdot n^{\frac{d-\sigma}{d}} \cdot \int_{\mathbb{R}^d}f(X)^{\frac{d-\sigma}{d}}d X,\]
	%\footnote{For two functions $g_1(n)$ and $g_2(n)$, we say $g_1(n)\sim g_2(n)$ if and only if
			%$\lim_{n\to \infty} {g_1(n)}/{g_2(n)}=1$.}
	provided $\Psi(x)\sim x^\sigma$, where $f(X)$ is the density of the absolutely continuous part of the distribution of the $\{X_i\}$.
\end{lem}

\begin{lem}[Kolmogorov's Strong LLN \cite{williams1991probability}]\label{lem-Kolmogorov-slln}
	
	Let $\{X_n\}$  be an i.i.d. sequence of random variables having finite mean: For $\forall n$,
	$\mathbf{E}[X_n] < \infty$.
	Then, a strong law of large numbers (LLN) applies to the sample mean:
	\[\bar{X}_n \stackrel{a.s.}{\longrightarrow} \mathbf{E}[X_n],\]
	where  $\stackrel{a.s.}{\longrightarrow}$ denotes \emph{almost sure convergence}.
\end{lem}

\subsection{Proof of Lemma \ref{lem-EMST-B-D}}\label{proof-lem-EMST-B-D}
\begin{proof}
	With probability $1$, it holds that
	\begin{center}
		$|\EMST(\mathcal{A}^\mathrm{I}_k)|=\Theta(L^\mathrm{I}_{\mathcal{P}}(\beta, d_k))$ for $d_k=\omega(1)$,
	\end{center}
	where $L^\mathrm{I}_{\mathcal{P}}(\beta, d_k)$ is defined in Eq.(\ref{eq-L-P-beta-9765}). Combining with the fact that \[|\EMST(\mathcal{P}^\mathrm{I}_{k})|\geq |\EMST(\mathcal{A}^\mathrm{I}_k)|,\] then, we get that
	\begin{equation*}
		|\EMST(\mathcal{P}^\mathrm{I}_{k})|=\Omega(L^\mathrm{I}_{\mathcal{P}}(\beta, d_k)).
	\end{equation*}
	Then, our focus turns to the derivation of $ L^\mathrm{I}_{\mathcal{P}}(\beta, d_k) $. Based on the value of $ \beta $, we have:

	(1) When $ 0 \leq\beta <1 $,
	\begin{equation*}
		\int_{\mathcal{O}}\sqrt{f_{X_0}(X)} dX =  \Theta\left(n^{\frac{\beta-1}{2}} \cdot \int_{\mathcal{O}}\frac{dX}{\left(|X-X_{0}|^{2}+1\right)^{\frac{\beta}{2}}}\right)
	\end{equation*}
	$~~~~~~~~~~~~~~~~~~~~~~~= \Theta\left(n^{\frac{\beta-1}{2}} \cdot n^{1-\frac{\beta}{2}}\right) = \Theta\left(\sqrt{n}\right) $.

	(2) When $ \beta=1 $,
	\begin{equation*}
		\int_{\mathcal{O}}\sqrt{f_{X_0}(X)}dX = \Theta\left(\frac{1}{\sqrt{\log n}}\cdot \int_{\mathcal{O}}\frac{dX}{\left(|X-X_{0}|^{2}+1\right)^{\frac{1}{2}}}\right)
	\end{equation*}
	$~~~~~~~~~~~~~~~~~~~~~~~= \Theta\left(\frac{1}{\sqrt{\log n}} \cdot \sqrt{n}\right) = \Theta\left(\sqrt{\frac{n}{\log n}}\right) $.
	
	(3) When $ \beta>1 $,
	\begin{equation*}
		\int_{\mathcal{O}}\sqrt{f_{X_0}(X)}dX = \Theta\left( \int_{\mathcal{O}}\frac{dX}{\left(|X-X_{0}|^{2}+1\right)^{\frac{\beta}{2}}}\right).
	\end{equation*}
	
	Especially,
	
	when $ 1<\beta<2 $, $ \Theta\left( \int_{\mathcal{O}}\frac{dX}{\left(|X-X_{0}|^{2}+1\right)^{\frac{\beta}{2}}}\right) = \Theta\left(n^{1-\frac{\beta}{2}}\right) $;
	
	when $ \beta=2 $, $ \Theta\left( \int_{\mathcal{O}}\frac{dX}{\left(|X-X_{0}|^{2}+1\right)}\right) $=$ \Theta\left(\log n\right) $;
	
	when $ \beta>2 $, $ \Theta\left( \int_{\mathcal{O}}\frac{dX}{\left(|X-X_{0}|^{2}+1\right)^{\frac{\beta}{2}}}\right) $=$ \Theta\left(1\right) $.
	
	Combining with all cases above, we complete the proof.
\end{proof}

\section{Some Results}\label{our-reslts}
Here, we summary the results of complete form.
\subsection{Lower Bounds on $ \sum\nolimits_{k=1}^{n}|\mathrm{EMST}(\mathcal{P}^\mathrm{I}_k)|$}\label{lower-bound-E}
\begin{table*}[!t]
	
	\centering
	\caption{Lower Bounds on $ \sum\nolimits_{k=1}^{n}|\mathrm{EMST}(\mathcal{P}^\mathrm{I}_k)|$}
	\label{tab-lower-bound-EMST}
	\scalebox{0.7}
	{
		%\begin{tiny}
		\begin{tabular}{|p{1.8cm}||p{3.85cm}|p{3.85cm}|p{3.85cm}|p{3.85cm}|p{3.85cm}|}
			\hline
			$\varphi$ $\backslash$ $\beta$ & $\beta>2$ & $\beta=2$ & $ 1<\beta<2 $ & $\beta=1$ & $0\leq\beta<1$ \\
			\hline
			\hline

			$\varphi>\frac{3}{2}$ &
			$ \Omega(n)$ , $\gamma\geq0$; &
			$ \Omega(n \cdot \log n)$ , $\gamma\geq0$; &
			$ \Omega(n^{2-\frac{\beta}{2}})$ , $\gamma\geq0$; &
			$ \Omega(n^{\frac{3}{2}} / \sqrt{\log n})$ , $\gamma\geq0$; &
			$ \Omega(n^{\frac{3}{2}})$ , $\gamma\geq0$. \\
			\hline
			
			$\varphi=\frac{3}{2}$ & $\left\{
			\begin{array}{ll}
				\Omega(n)  ,   \\
				\qquad \gamma>1; \\
				\Omega(n \cdot \log n)  ,  \\
				\qquad 0\leq\gamma\leq1.\\
			\end{array}
			\right. $ &
			$\left\{
			\begin{array}{ll}
				\Omega(n \cdot \log n)  ,   \\
				\qquad \gamma>1; \\
				\Omega(n \cdot (\log n)^2)  ,  \\
				\qquad 0\leq\gamma\leq1.\\
			\end{array}
			\right. $ &
			$\left\{
			\begin{array}{ll}
				\Omega(n^{2-\frac{\beta}{2}})  ,   \\
				\qquad \gamma>1; \\
				\Omega(n^{2-\frac{\beta}{2}} \cdot \log n)  ,  \\
				\qquad 0\leq\gamma\leq1.\\
			\end{array}
			\right. $ &
			$\left\{
			\begin{array}{ll}
				\Omega(n^{\frac{3}{2}} / \sqrt{\log n})  ,   \\
				\qquad \gamma>1; \\
				\Omega(n^{\frac{3}{2}} \cdot \sqrt{\log n})  ,  \\
				\qquad  0\leq\gamma\leq1.\\
			\end{array}
			\right. $ &
			$\left\{
			\begin{array}{ll}
				\Omega(n^{\frac{3}{2}})  ,   \\
				\qquad \gamma>1; \\
				\Omega(n^{\frac{3}{2}} \cdot \log n)  ,  \\
				\qquad 0\leq\gamma\leq1.\\
			\end{array}
			\right. $  \\
			\hline
			
			$1<\varphi<\frac{3}{2}$ & $\left\{
			\begin{array}{ll}
				\Omega(n)  ,   \\
				\qquad \gamma>\frac{5}{2}-\varphi;\\
				\Omega(n \cdot \log n) , \\
				\qquad \gamma=\frac{5}{2}-\varphi;  \\
				\Omega(n^{\frac{7}{2}-\gamma-\varphi}) , \\
				\qquad 1<\gamma<\frac{5}{2}-\varphi;  \\
				\Omega(n^{\frac{5}{2}-\varphi} / \log n) , \\
				\qquad \gamma=1;  \\
				\Omega(n^{\frac{5}{2}-\varphi})  ,  \\
				\qquad 0\leq\gamma<1.\\
			\end{array}
			\right. $ &
			$\left\{
			\begin{array}{ll}
				\Omega(n \cdot \log n)  ,   \\
				\qquad \gamma>\frac{5}{2}-\varphi;\\
				\Omega(n \cdot (\log n)^2) , \\
				\qquad \gamma=\frac{5}{2}-\varphi;  \\
				\Omega(n^{\frac{7}{2}-\gamma-\varphi} \cdot \log n) , \\
				\qquad 1<\gamma<\frac{5}{2}-\varphi;  \\
				\Omega(n^{\frac{5}{2}-\varphi}) , \\
				\qquad \gamma=1;  \\
				\Omega(n^{\frac{5}{2}-\varphi} \cdot \log n)  ,  \\
				\qquad 0\leq\gamma<1.\\
			\end{array}
			\right. $ &
			$\left\{
			\begin{array}{ll}
				\Omega(n^{2-\frac{\beta}{2}})  ,   \\
				\qquad \gamma>\frac{5}{2}-\varphi;\\
				\Omega(n^{2-\frac{\beta}{2}} \cdot \log n) , \\
				\qquad \gamma=\frac{5}{2}-\varphi;  \\
				\Omega(n^{\frac{9}{2}-\gamma-\varphi-\frac{\beta}{2}}) , \\
				\qquad 1<\gamma<\frac{5}{2}-\varphi;  \\
				\Omega(n^{\frac{7}{2}-\varphi-\frac{\beta}{2}} / \log n) , \\
				\qquad \gamma=1;  \\
				\Omega(n^{\frac{7}{2}-\varphi-\frac{\beta}{2}})  ,  \\
				\qquad 0\leq\gamma<1.\\
			\end{array}
			\right. $ &
			$\left\{
			\begin{array}{ll}
				\Omega(n^{\frac{3}{2}} / \sqrt{\log n})  ,   \\
				\qquad \gamma>\frac{5}{2}-\varphi;\\
				\Omega(n^{\frac{3}{2}} \cdot \sqrt{\log n}) , \\
				\qquad \gamma=\frac{5}{2}-\varphi;  \\
				\Omega(n^{4-\gamma-\varphi} / \sqrt{\log n}) , \\
				\qquad 1<\gamma<\frac{5}{2}-\varphi;  \\
				\Omega(n^{3-\varphi} / (\log n)^{\frac{3}{2}}) , \\
				\qquad \gamma=1;  \\
				\Omega(n^{3-\varphi} / \sqrt{\log n})  ,  \\
				\qquad 0\leq\gamma<1.\\
			\end{array}
			\right. $ &
			$\left\{
			\begin{array}{ll}
				\Omega(n^{\frac{3}{2}})  ,   \\
				\qquad \gamma>\frac{5}{2}-\varphi;\\
				\Omega(n^{\frac{3}{2}} \cdot \log n) , \\
				\qquad \gamma=\frac{5}{2}-\varphi;  \\
				\Omega(n^{4-\gamma-\varphi}) , \\
				\qquad 1<\gamma<\frac{5}{2}-\varphi;  \\
				\Omega(n^{3-\varphi} / \log n) , \\
				\qquad \gamma=1;  \\
				\Omega(n^{3-\varphi})  ,  \\
				\qquad 0\leq\gamma<1.\\
			\end{array}
			\right. $ \\
			\hline
			
			$\varphi=1$ & $\left\{
			\begin{array}{ll}
				\Omega(n)  , \\
				\qquad  \gamma\geq\frac{3}{2}; \\
				\Omega(n^{\frac{5}{2}-\gamma} / \log n) , \\
				\qquad 1<\gamma<\frac{3}{2};  \\
				\Omega(n^{\frac{3}{2}} / (\log n)^2) , \\
				\qquad \gamma=1;  \\
				\Omega(n^{\frac{3}{2}} / \log n)  , \\
				\qquad  0\leq\gamma<1.\\
			\end{array}
			\right. $ &
			$\left\{
			\begin{array}{ll}
				\Omega(n \cdot \log n)  , \\
				\qquad  \gamma\geq\frac{3}{2}; \\
				\Omega(n^{\frac{5}{2}-\gamma}) , \\
				\qquad 1<\gamma<\frac{3}{2};  \\
				\Omega(n^{\frac{3}{2}} / \log n) , \\
				\qquad \gamma=1;  \\
				\Omega(n^{\frac{3}{2}})  , \\
				\qquad  0\leq\gamma<1.\\
			\end{array}
			\right. $ &
			$\left\{
			\begin{array}{ll}
				\Omega(n^{2-\frac{\beta}{2}})  , \\
				\qquad  \gamma\geq\frac{3}{2}; \\
				\Omega(n^{\frac{7}{2}-\gamma-\frac{\beta}{2}} / \log n) , \\
				\qquad  1<\gamma<\frac{3}{2};  \\
				\Omega(n^{\frac{5}{2}-\frac{\beta}{2}} / (\log n)^2) , \\
				\qquad \gamma=1;  \\
				\Omega(n^{\frac{5}{2}-\frac{\beta}{2}} / \log n)  , \\
				\qquad  0\leq\gamma<1.\\
			\end{array}
			\right. $ &
			$\left\{
			\begin{array}{ll}
				\Omega(n^{\frac{3}{2}} / \sqrt{\log n})  , \\
				\qquad  \gamma\geq\frac{3}{2}; \\
				\Omega(n^{3-\gamma} / (\log n)^{\frac{3}{2}}) , \\
				\qquad 1<\gamma<\frac{3}{2};  \\
				\Omega(n^{2} / (\log n)^\frac{5}{2}) , \\
				\qquad  \gamma=1;  \\
				\Omega(n^{2} / (\log n)^\frac{3}{2})  , \\
				\qquad  0\leq\gamma<1.\\
			\end{array}
			\right. $ &
			$\left\{
			\begin{array}{ll}
				\Omega(n^{\frac{3}{2}})  , \\
				\qquad  \gamma\geq\frac{3}{2}; \\
				\Omega(n^{3-\gamma} / \log n) , \\
				\qquad  1<\gamma<\frac{3}{2};  \\
				\Omega(n^{2} / (\log n)^2) , \\
				\qquad  \gamma=1;  \\
				\Omega(n^{2} / \log n)  , \\
				\qquad  0\leq\gamma<1.\\
			\end{array}
			\right. $ \\
			\hline
			
			$0\leq\varphi<1$ & $\left\{
			\begin{array}{ll}
				\Omega(n)  , \\
				\qquad  \gamma>\frac{3}{2}; \\
				\Omega(n \cdot \log n)  , \\
				\qquad  \gamma=\frac{3}{2}; \\
				\Omega(n^{\frac{5}{2}-\gamma}) , \\
				\qquad 1<\gamma<\frac{3}{2};  \\
				\Omega(n^{\frac{3}{2}} / \log n) , \\
				\qquad  \gamma=1;  \\
				\Omega(n^{\frac{3}{2}})  , \\
				\qquad  0\leq\gamma<1.\\
			\end{array}
			\right. $ &
			$\left\{
			\begin{array}{ll}
				\Omega(n \cdot \log n)  , \\
				\qquad  \gamma>\frac{3}{2}; \\
				\Omega(n \cdot (\log n)^2)  , \\
				\qquad  \gamma=\frac{3}{2}; \\
				\Omega(n^{\frac{5}{2}-\gamma} \cdot \log n) , \\
				\qquad  1<\gamma<\frac{3}{2};  \\
				\Omega(n^{\frac{3}{2}}) , \\
				\qquad  \gamma=1;  \\
				\Omega(n^{\frac{3}{2}} \cdot \log n)  , \\
				\qquad  0\leq\gamma<1.\\
			\end{array}
			\right. $ &
			$\left\{
			\begin{array}{ll}
				\Omega(n^{2-\frac{\beta}{2}})  , \\
				\qquad  \gamma>\frac{3}{2}; \\
				\Omega(n^{2-\frac{\beta}{2}} \cdot \log n)  , \\
				\qquad  \gamma=\frac{3}{2}; \\
				\Omega(n^{\frac{7}{2}-\gamma-\frac{\beta}{2}}) , \\
				\qquad 1<\gamma<\frac{3}{2};  \\
				\Omega(n^{\frac{5}{2}-\frac{\beta}{2}} / \log n) , \\
				\qquad  \gamma=1;  \\
				\Omega(n^{\frac{5}{2}-\frac{\beta}{2}})  , \\
				\qquad  0\leq\gamma<1.\\
			\end{array}
			\right. $ &
			$\left\{
			\begin{array}{ll}
				\Omega(n^{\frac{3}{2}} / \sqrt{\log n})  , \\
				\qquad  \gamma>\frac{3}{2}; \\
				\Omega(n^{\frac{3}{2}} \cdot \sqrt{\log n})  , \\
				\qquad  \gamma=\frac{3}{2}; \\
				\Omega(n^{3-\gamma} / \sqrt{\log n}) , \\
				\qquad 1<\gamma<\frac{3}{2};  \\
				\Omega(n^{2} / (\log n)^{\frac{3}{2}}) , \\
				\qquad  \gamma=1;  \\
				\Omega(n^{2} / \sqrt{\log n})  , \\
				\qquad  0\leq\gamma<1.\\
			\end{array}
			\right. $ &
			$\left\{
			\begin{array}{ll}
				\Omega(n^{\frac{3}{2}})  , \\
				\qquad  \gamma>\frac{3}{2}; \\
				\Omega(n^{\frac{3}{2}} \cdot \log n)  , \\
				\qquad  \gamma=\frac{3}{2}; \\
				\Omega(n^{3-\gamma}) , \\
				\qquad  1<\gamma<\frac{3}{2};  \\
				\Omega(n^{2} / \log n) , \\
				\qquad  \gamma=1;  \\
				\Omega(n^{2})  , \\
				\qquad  0\leq\gamma<1.\\
			\end{array}
			\right. $ \\
			\hline
		\end{tabular}
		%\end{tiny}
	}
\end{table*}

\subsection{Lower Bounds on The Derived Traffic Load $\mathrm{L}_{\mathbb{N}}^{\mathrm{I}} $}\label{lower-bound-L}
Within the Table \ref{G-tab-total}, we have highlighted the situations where each law holds true under the condition $\lambda=\Theta(1)$. Metcalfe's law is distinguished with a vibrant yellow background, while Sarnoff's law is denoted by a soothing blue background, and Odlyzko's law is represented with an invigorating green background. By carefully analyzing the conditions presented in the table, we can unravel the intricate and diverse nature of scenarios in which Metcalfe's law proves to be both applicable and valid.
